# Supplementary material for: Quantized Self-Assembly of Discotic Rings in a Liquid Crystal Confined in Nanopores
Source: arXiv:1801.07605 ancillary file (2018-01-23)
Supplement: Supplementary file 1 [file Sentker-SM-2017-11-10.pdf]

# Supplemental Material:

## Quantized Self-Assembly of Discotic Rings in a Liquid Crystal Confined in Nanopores

Kathrin Sentker,<sup>1</sup> Arne W. Zantop,<sup>2</sup> Milena Lippmann,<sup>3</sup> Tommy Hofmann,<sup>4</sup> Oliver H. Seeck,<sup>3</sup> Andriy V. Kityk,<sup>5</sup> Arda Yildirim,<sup>6</sup> Andreas Schönhalz,<sup>6</sup> Marco G. Mazza,<sup>2</sup> and Patrick Huber<sup>1,\*</sup>

<sup>1</sup>*Institut für Materialphysik und -technologie, Technische Universität Hamburg, Eißendorferstr. 42, D-21073 Hamburg, Germany*

<sup>2</sup>*Max-Planck-Institut für Dynamik und Selbstorganisation, Am Faßberg 17, D-37077 Göttingen, Germany*

<sup>3</sup>*Deutsches Elektronen Synchrotron, Notkestraße 85, D-22607 Hamburg, Germany*

<sup>4</sup>*Helmholtz-Zentrum Berlin für Materialien und Energie, Hahn-Meitner-Platz 1, D-14109 Berlin, Germany*

<sup>5</sup>*Faculty of Electrical Engineering, Czestochowa University of Technology, Al. Armii Krajowej 17, P-42-200 Czestochowa, Poland*

<sup>6</sup>*Bundesanstalt für Materialforschung und -prüfung, Unter den Eichen 87, D-12205 Berlin, Germany*

(Dated: January 22, 2018)

### I. SAMPLE PREPARATION & X-RAY DIFFRACTION EXPERIMENT

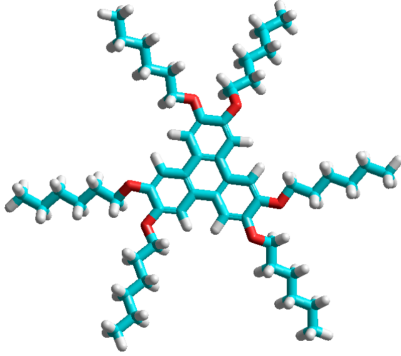

FIG. I.1. Chemical structure of HAT6.

Porous silica (pSiO<sub>2</sub>) was fabricated by an electrochemical anodic etching procedure of silicon wafers and a subsequent oxidation process[1, 2]. Highly p-doped <100> silicon wafer with a resistivity of  $R = 0.01 - 0.02 \, \Omega\text{cm}$  were etched in an electrolyte of 40% hydrofluoric acid (48% concentrated) and 60% ethanol with an etching current density of  $J = 13.3 \, \text{mA/cm}^2$  applied for 8 h [3]. The resulting 360  $\mu\text{m}$  thick membrane was oxidized at 800°C for 48 h. The pSiO<sub>2</sub> surface naturally enforces face-on anchoring. Surface treatment with a 1:9 dimethylchlorosilan-trichloromethane solution for 2 h replaces the hydrophilic hydroxyl groups by hydrophobic methyl groups, creating edge-on surface anchoring conditions. This treatment enhances the surface contact angle from 37° to 103° corresponding to a hydrophobic surface. Volumetric nitrogen sorption isotherms yield a pore diameter  $d = 17 \, \text{nm}$  and porosity of  $P = 51\%$ . After filling the membranes with

2,3,6,7,10,11-hexakis(hexyloxy)triphenylene (HAT6) via spontaneous imbibition [4] the surface is scratched carefully to remove any remaining material on top.

The transmission synchrotron X-ray experiment, see the schematic in Fig. I was performed at the P08 beamline of the PETRA III synchrotron (DESY) with a beam size of  $(V \times H) = (30 \times 100) \, \mu\text{m}^2$ ,  $\lambda = 0.496 \, \text{\AA}$ , a Perkin Elmer detector and temperatures in the interval 380 – 310 K. The rotation angle  $\omega$  of the membrane normal and thus the pore axis with respect to the incident beam direction was chosen as close as possible to 90°, i.e.  $\omega = 75^\circ$ . Thereby, we confined in a maximal manner the wave vector transfers within planes aligned parallel to the pore axes, without shadowing scattering directions in a  $q$ -range up to the intracolumnar order,  $q_{dd} = (1.726 \pm 0.008) \, \text{\AA}^{-1}$ . However, the wave vector transfers have still small contributions within planes aligned perpendicular to the pore axes. They are tacitly neglected in the discussions of the reciprocal space pictures in the manuscript. Most prominently the deviation from  $\omega = 90^\circ$  leads to a deviation of the streaks typical of the intracolumnar order from a perfect polar centering. A few sharp Bragg rings typical of the aluminum foil used to achieve a good thermalization of the membrane as well as the broad first maximum of the structure factor of the amorphous silica pore walls were detected at wave vector transfers  $q_{Al1} = (1.411 \pm 0.005) \, \text{\AA}^{-1}$ ,  $q_{Al2} = (1.576 \pm 0.002) \, \text{\AA}^{-1}$ ,  $q_{Al3} = (1.726 \pm 0.005) \, \text{\AA}^{-1}$  and  $q_{SiO2} = (1.4896 \pm 0.005) \, \text{\AA}^{-1}$  and thus constitute a temperature-independent scattering background. The intensities typical of the intra- and intercolumnar order are by contrast strongly temperature-dependent as discussed in the manuscript.

### II. MODEL AND COMPUTATIONAL DETAILS

The Gay-Berne-II (GBII) model potential energy [5, 6] for two molecules at positions  $\mathbf{r}_i$  and  $\mathbf{r}_j$ , separated by a distance  $\mathbf{r}_{ij} \equiv \mathbf{r}_i - \mathbf{r}_j$ , and with orientations denoted by

\* patrick.huber@tuhh.de

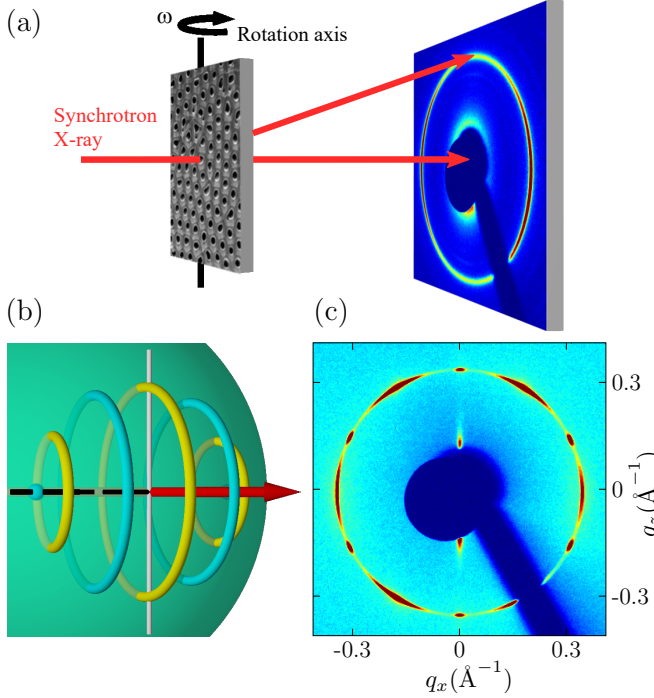

FIG. I.2. (a) Schematics of the X-ray scattering experiment (b) Reciprocal space typical of  $\{10\}$  and  $\{11\}$  orientational domains of hexagonal arranged circular rings, as depicted in Fig. 2(a). The dashed and red arrow indicate the pore axis and the incident beam direction, respectively. The reciprocal pattern cuts into the Ewald sphere at 12 points, and thus results in a 12-fold diffraction pattern. (c) Diffraction pattern of HAT6 confined in parallel cylindrical pores of edge-on, surface-grafted anodic alumina oxide membrane with 95 nm pore diameter at  $T=348$  K, recorded in a scattering geometry as described above. Except for a slight variation in the azimuthal alignment of the  $\{11\}$  domains, it agrees with the scattering pattern described in (a) and thus evidences the existence of both hexagonal orientational domains.

the unit vectors  $\hat{\mathbf{e}}_i$  and  $\hat{\mathbf{e}}_j$ , respectively, reads

$$U(\mathbf{r}_{ij}, \hat{\mathbf{e}}_i, \hat{\mathbf{e}}_j) = 4 \epsilon(\hat{\mathbf{r}}_{ij}, \hat{\mathbf{e}}_i, \hat{\mathbf{e}}_j) \times \left\{ \left[ \frac{\sigma_{\text{ff}}}{r_{ij} - \sigma(\hat{\mathbf{r}}_{ij}, \hat{\mathbf{e}}_i, \hat{\mathbf{e}}_j) + \sigma_{\text{ff}}} \right]^{12} - \left[ \frac{\sigma_{\text{ff}}}{r_{ij} - \sigma(\hat{\mathbf{r}}_{ij}, \hat{\mathbf{e}}_i, \hat{\mathbf{e}}_j) + \sigma_{\text{ff}}} \right]^6 \right\}, \quad (\text{S1})$$

with the orientation-dependent energy scale function

$$\epsilon(\hat{\mathbf{r}}_{ij}, \hat{\mathbf{e}}_i, \hat{\mathbf{e}}_j) = \epsilon_0 \epsilon'_{\text{f}}(\hat{\mathbf{r}}_{ij}, \hat{\mathbf{e}}_i, \hat{\mathbf{e}}_j) \epsilon''_{\text{f}}(\hat{\mathbf{r}}_{ij}, \hat{\mathbf{e}}_i, \hat{\mathbf{e}}_j), \quad (\text{S2})$$

$$\epsilon_1(\hat{\mathbf{r}}_{ij}, \hat{\mathbf{e}}_i, \hat{\mathbf{e}}_j) = [1 - \chi^2(\hat{\mathbf{e}}_i \cdot \hat{\mathbf{e}}_j)^2]^{-1/2}, \quad (\text{S3})$$

$$\epsilon_2(\hat{\mathbf{r}}_{ij}, \hat{\mathbf{e}}_i, \hat{\mathbf{e}}_j) = \left\{ 1 - \frac{\chi'}{2} \left[ \frac{(\hat{\mathbf{r}}_{ij} \cdot \hat{\mathbf{e}}_i + \hat{\mathbf{r}}_{ij} \cdot \hat{\mathbf{e}}_j)^2}{1 + \chi'(\hat{\mathbf{e}}_i \cdot \hat{\mathbf{e}}_j)} + \frac{(\hat{\mathbf{r}}_{ij} \cdot \hat{\mathbf{e}}_i - \hat{\mathbf{r}}_{ij} \cdot \hat{\mathbf{e}}_j)^2}{1 - \chi'(\hat{\mathbf{e}}_i \cdot \hat{\mathbf{e}}_j)} \right] \right\}, \quad (\text{S4})$$

and the orientation-dependent effective radius function

$$\sigma(\hat{\mathbf{r}}_{ij}, \hat{\mathbf{e}}_i, \hat{\mathbf{e}}_j) = \sigma_0 \left\{ 1 - \frac{\chi}{2} \left[ \frac{(\hat{\mathbf{r}}_{ij} \cdot \hat{\mathbf{e}}_i + \hat{\mathbf{r}}_{ij} \cdot \hat{\mathbf{e}}_j)^2}{1 + \chi(\hat{\mathbf{e}}_i \cdot \hat{\mathbf{e}}_j)} + \frac{(\hat{\mathbf{r}}_{ij} \cdot \hat{\mathbf{e}}_i - \hat{\mathbf{r}}_{ij} \cdot \hat{\mathbf{e}}_j)^2}{1 - \chi(\hat{\mathbf{e}}_i \cdot \hat{\mathbf{e}}_j)} \right] \right\}^{-1/2}. \quad (\text{S5})$$

In Eq. (S1)-(S5),  $r_{ij} = |\mathbf{r}_{ij}|$ ,  $\sigma_0$  and  $\epsilon_0$  are the units of length and energy, respectively. The molecules' spatial extent leads to minimum face-to-face distance  $\sigma_{\text{ff}}$  and minimum edge-to-edge distance  $\sigma_{\text{ee}}$ . The parameter  $\chi = \frac{\kappa^2 - 1}{\kappa^2 + 1}$ ,  $\kappa \equiv \sigma_{\text{ff}}/\sigma_{\text{ee}}$ ,  $\sigma_{\text{ee}} = \sigma_0$ , determines the shape anisotropy of the discotic molecule, and  $\chi' = \frac{\kappa'^{1/\mu} - 1}{\kappa'^{1/\mu} + 1}$ ,  $\kappa' \equiv \epsilon_{\text{ee}}/\epsilon_{\text{ff}}$ , determines the energy anisotropy of the discotic molecule, and the subscripts 'ee' and 'ff' refer to the 'edge-to-edge' and 'face-to-face' configurations, respectively. We fix the values of the exponents  $\mu = 1$  and  $\nu = 2$ , and neglect molecular interactions for molecules separated by a distance larger than  $r_c = 2.5\sigma_0$ . We also fix  $\kappa = 0.2$  and  $\kappa' = 0.2$ , suitable for HAT6. This set of parameters leads to the formation of isotropic, nematic, columnar and crystalline phases depending on the pressure and temperature applied to the molecular system [6].

To realize the cylindrical confinement, we implement walls using both energetically and spatially anisotropic fluid particle-wall interaction energy

$$U_{\text{fw}}(\mathbf{r}_i, \hat{\mathbf{e}}_i) = \epsilon_{\text{fw}} \left\{ \frac{2}{15} \left[ \frac{\sigma_{\text{ff}}}{r_{i\text{w}} - \sigma_{\text{w}}(\hat{\mathbf{e}}_i)} \right]^9 - [(\hat{\mathbf{n}}_{\text{w}} \times \hat{\mathbf{e}}_i) \cdot \hat{\mathbf{z}}]^2 \left[ \frac{\sigma_{\text{ff}}}{r_{i\text{w}} - \sigma_{\text{w}}(\hat{\mathbf{e}}_i)} \right]^3 \right\} \quad (\text{S6})$$

for a particle separated by distance  $r_{i\text{w}}$  from the wall, whose local normal is  $\hat{\mathbf{n}}_{\text{w}}$ , and with

$$\sigma_{\text{w}}(\hat{\mathbf{e}}_i) = \frac{\sigma_0}{2} \left\{ \left[ 1 - \frac{2\chi_{\text{w}}(\hat{\mathbf{n}}_{\text{w}} \cdot \hat{\mathbf{e}}_i)^2}{1 + \chi_{\text{w}}} \right]^{-1/2} - \kappa \right\}, \quad (\text{S7})$$

where ' $\times$ ' denotes the vector product. The fluid-wall interaction energy in Eq. (S6) induces an edge-on anchoring to the wall surface, along the nanopore axis, which we conventionally align to the  $z$ -axis. When a fluid molecule interacts with the confining wall we halve the shape anisotropy by using

$$\chi_{\text{w}} = \frac{4\kappa^2 - 1}{4\kappa^2 + 1}$$

as a modified version of the parameter  $\chi$  of the fluid-fluid interaction energy. A similar fluid-wall interaction model was used in a study by Caprion [7]. We use a moderate wall interaction strength of  $\epsilon_{\text{fw}} = 8\epsilon_0$  and cut-off length of  $2.5\sigma_{\text{ee}}$  also for the fluid-wall interactions.

For the simulation of an expanded ensemble, we employ parallel tempering [8] and consider a set of reciprocal temperatures  $\beta_m = 1/k_{\text{B}}T_m$ ,  $m = 1, \dots, N_{\text{R}}$ , where

$k_B$  is the Boltzmann constant and  $T_m$  are temperatures, and use an expansion of the isothermal-isobaric ensemble (NPT) [9, 10]. This gives us a swapping probability between the configurations  $x_m, x_{m+1}$  of two neighbouring temperatures  $\beta_m, \beta_{m+1}$  of  $p_{\text{acc}}(x_m \leftrightarrow x_{m+1}) = \exp[\Delta\beta(\Delta E + P\Delta V)]$ .

We implemented the method for parallel simulation using up to  $N_R = 96$  reciprocal temperatures  $\beta_m$  running on different CPUs that communicate via Message Passing Interface (MPI). At each temperature a replica of the  $N$  molecule system is simulated. At the start of each simulation, all replicas are initialised with a different random molecular configuration (positions and orientations). The simulation is carried out in the following manner: firstly, for each replica  $(6N + 3)$  standard NPT Monte-Carlo steps are performed, secondly a replica exchange is attempted between a randomly selected pair of replicas with consecutive temperatures. After 500000 such steps, we start collecting ensemble averages.

We performed simulations with a nanopore of diameter  $11.25\sigma_{\text{ee}}$  filled with  $N = 4000$  particles. We simulate at a reduced pressure of  $P\sigma_0^3/\epsilon_0 = 50$  where the GBII model exhibits nematic, columnar, and crystalline phases upon variation of the temperature.

### III. ORDER PARAMETERS

The presence of confining walls in a discotic liquid crystal causes  $\hat{\mathbf{n}}(\mathbf{r})$  to deviate from a constant  $\hat{\mathbf{n}}_0$ . Associated with this deformation of  $\hat{\mathbf{n}}(\mathbf{r})$  is a local deviation between the nematic order parameter and its bulk value in the absence of any confinement. Both, deformation of  $\hat{\mathbf{n}}(\mathbf{r})$  and the associated variation of  $S(\mathbf{r})$  cause changes in the free energy of the nanoconfined system. Adopting a coarse-grained, continuum perspective a key quantity is the local alignment tensor  $\mathbf{Q}(\mathbf{r})$  whose components can be cast as

$$Q_{\alpha\beta}(\mathbf{r}) = \frac{S(\mathbf{r})}{2} [3n_\alpha(\mathbf{r})n_\beta(\mathbf{r}) - \delta_{\alpha\beta}] \quad (\text{S8})$$

where  $S(\mathbf{r})$  is the nematic order parameter,  $n_\alpha(\mathbf{r})$  is the  $\alpha$ -component of  $\hat{\mathbf{n}}(\mathbf{r})$ , and  $\delta_{\alpha\beta}$  is the Kronecker symbol. The assumption underlying Eq. (S8) is that a spatial variation of the degree of nematic order of uniaxial symmetry and a deformation of the nematic director field are coupled.  $\mathbf{Q}(\mathbf{r})$  is a real, symmetric, and traceless second-rank tensor which can be represented by a  $3 \times 3$  matrix.

To calculate the local nematic order parameter one has to solve the eigenvalue equation  $\mathbf{Q}(\mathbf{r}) \cdot \hat{\mathbf{n}}_n(\mathbf{r}) = \lambda_n(\mathbf{r})\hat{\mathbf{n}}_n(\mathbf{r})$  where  $\lambda_n$  is the  $n$ th eigenvalue and  $\hat{\mathbf{n}}_n(\mathbf{r})$  the associated eigenvector. The three eigenvalues  $\lambda_-(\mathbf{r}) < \lambda_0(\mathbf{r}) < \lambda_+(\mathbf{r})$  can be obtained analytically using Cardano's formula. One can define the local nematic order parameter  $S(\mathbf{r})$  as the largest eigenvalue  $\lambda_+(\mathbf{r})$  and the associated eigenvector as the local director  $\hat{\mathbf{n}}(\mathbf{r})$ .

To investigate the nature of the local molecular order during the individual transitions, we employ the spatially resolved bond orientational order parameters in the implementation of Lechner and Dellago [11] that achieves a high accuracy in the determination of the local symmetries. The average local bond order parameters are defined as

$$\bar{q}_l(i) = \sqrt{\frac{4\pi}{2l+1} \sum_{m=-l}^l |\bar{q}_{lm}(i)|^2} \quad (\text{S9})$$

where

$$\bar{q}_{lm}(i) = \frac{1}{\tilde{N}_b(i)} \sum_{k=0}^{\tilde{N}_b(i)} q_{lm}(k), \quad (\text{S10})$$

and the local orientational order vectors are defined as usual

$$q_{lm}(i) = \frac{1}{N_b(i)} \sum_{j=1}^{N_b(i)} Y_{lm}(\mathbf{r}_{ij}) \quad (\text{S11})$$

where  $Y_{lm}(\mathbf{r}_{ij})$  are the spherical harmonics,  $N_b(i)$  is the set of nearest neighbors of particle  $i$ , and  $\tilde{N}_b(i) = N_b(i) \cup \{i\}$ .

The snapshots are visualized with the molecular visualization software QMGA.

- 
- [1] M. J. Sailor, *Porous Silicon in Practice - Preparation, Characterization and Applications* (Wiley-VCH, Weinheim, 2011).
  - [2] L. Canham, *Handbook of Porous Silicon*, edited by L. Canham (Springer, 2015).
  - [3] S. Gruener and P. Huber, Phys. Rev. Lett. **100**, 064502 (2008).
  - [4] S. Gruener and P. Huber, J. Phys. : Cond. Matt. **23**, 184109 (2011).
  - [5] M. A. Bates and G. R. Luckhurst, J. Chem. Phys. **104**, 6696 (1996).
  - [6] D. Caprion, L. Bellier-Castella, and J.-P. Ryckaert, Phys. Rev. E **67**, 041703 (2003).
  - [7] D. Caprion, Eur. Phys. J. E **28**, 305 (2009).
  - [8] R. H. Swendsen and J.-S. Wang, Phys. Rev. Lett. **57**, 2607 (1986).
  - [9] Q. Yan and J. J. de Pablo, J. Chem. Phys. **111**, 9509 (1999).
  - [10] D. J. Earl and M. W. Deem, Phys. Chem. Chem. Phys. **7**, 3910 (2005).
  - [11] W. Lechner and C. Dellago, J. Chem. Phys. **129**, 114707 (2008).
